# Supplementary material for: Covariant Compositional Networks For Learning Graphs
Source: arXiv:1801.02144 source file (2018-01-07)
Supplement: Supplementary file 1 [file appendix_tensor.tex]

\Section{General Tensor Rules and Notation}

\subsection{Tensor Index Notation}
% TODO: this is just a slop of words
Indices that appear once in a tensor subscript are free variables.
Indices may occur no more than twice in a given term and indices
that occur more than twice are summed over.

The rank of a tensor is its number of free variables.
A free index varies over its range(IE: \m{i = 1, 2, ..., n}). Expressions of
the form: $A_{i_1, ... i_k} = B_{i_1, ..., i_l}$, where each index varies
over \m{i_j = 1, 2, ..., n} can be understood as \m{n^k} separate equations
for each assignment of $i_j$ over its range. Each term in a valid
tensor expression must have the same set of free indices.

Repeated indices are summed over. This notation lends itself to
consise matrix and tensor operations. For example:
let \m{\mathbf{A} \in \mathbb{R}^{3 \cross 3}} we can equivalently
express it as: \m{\mathbf{A} = A_{ij}}
The matrix vector product \m{\mathbf{A} v}:
$$(\mathbf{A} v)_{i} = A_{ij} v_j$$

From section 4.2, we had the following claim:
the action \m{F_i \mapsto P_{\pi} F_i P_{\pi}^\top} is equivalent to the action:
\m{f_i \mapsto (P_\pi \otimes P_\pi) f_i}.

\begin{proof}

\end{proof}
